# Supplementary material for: Exploring Large Language Models for Hate Speech Detection in Rioplatense Spanish
Source: arXiv:2410.12174 source file (2024-10-16)
Supplement: Supplementary file 1 [file appendix.tex]

\section{Dataset information}
\label{app:ddd}

\begin{table*}[t]
    \centering
    \small
    \begin{tabular}{l p{0.5\textwidth} p{0.3\textwidth}}
        Category              & Context                                                                                                  & Comment                                \\
        \hline
        WOMEN                 & Mia Khalifa: acted in porn videos for a few months, became world famous and now fights to erase her past & @usuario HAHAHA KEEP SUCKING....       \\
        \rule{0pt}{3ex}LGBTI  & The story of the Colombian trans model kissing the belly of her eight-month pregnant husband             & @usuario A male kissing another male   \\

        \rule{0pt}{3ex}RACISM & Yanzhong Huang: ``It is quite likely that a Covid-21 is already brewing''                                & @user Urgent bombs to that damned race \\
        \rule{0pt}{3ex} CLASS & Social movements cut off 9 de Julio Av.: they demand a minimum wage of \$45,000                          & @user get to work, mfs                 \\                                                                                                                              \\
        \hline
    \end{tabular}
    \caption{Hateful examples from the analyzed dataset \cite{perez2023assessing}.}
    \label{tab:dataset_examples}
\end{table*}

Table \ref{tab:dataset_examples} illustrates some of the examples from the dataset. The context is the news tweet, and the comment is the user's reaction to it. The comment is the one that is labeled as hateful or not. Each comment might have more than one label, as it might be hateful for more than one characteristic (e.g. \textit{racism} and \textit{class}).
